# Supplementary material for: Winding Clearness for Differentiable Point Cloud Optimization
Source: arXiv:2401.13639 source file (2025-07-31)
Supplement: Supplementary file 1 [file Supplementary.pdf]

# Supplementary Material

## A THE IMPORTANCE OF THE REGULARIZATION TERM $R(P)$

In this section, we aim to explicate the significance of the regularization term  $R(P)$  in Equation (14) of the original manuscript. An alternative approach for computing the surfels  $\mu$  in Section 4 is concatenating the matrix  $A_1(P)$  of point constraints and  $A_2(P)$  of boundary constraints, and obtain a square matrix  $C(P)$  as follows:

$$C(P) = (A_1^T(P), A_2^T(P))^T. \quad (1)$$

Additionally, we define  $c = (1/2, 1/2, \dots, 0, 0, \dots, 0)^T$  as a vector with the first  $N$  values to  $1/2$ , and the remaining values to 0. Subsequently, the surfels  $\mu$  can be solved by the following equation:

$$C(P)\mu = c. \quad (2)$$

If  $C(P)$  is invertible, the surfels  $\mu$  can be computed as  $\mu = C^{-1}(P)c$ . In this case, the winding clearness error will always be zero. However, it becomes challenging to generate a smooth and reliable winding number field without including the regularization term  $R(P)$ , which controls the magnitude of  $\mu$ . If the solution of Equation (2) yields high magnitudes for  $\mu$ , it contradicts the meaning of the surfel. In this case, the generated function cannot represent the winding number field of this point cloud, i.e., 1 inside and 0 outside. This phenomenon is demonstrated in Fig. 1, where we show the implicit field generated by a 2D circle of  $\sigma = 0.001$  with (a) and without (b) the regularization term  $R(P)$ . We can observe in Fig. 1 (b) that the function becomes jagged and unreliable if we solve Equation (2) directly. Fig. 1 (a) illustrates the results of incorporating the regularization term  $R(P)$  in the formulation, which highlights the necessity of  $R(P)$  in creating a viable winding number field. If Equation (2) above is also regularized and formulated as a least squares problem, it shares similarities with the formulation in the original manuscript.

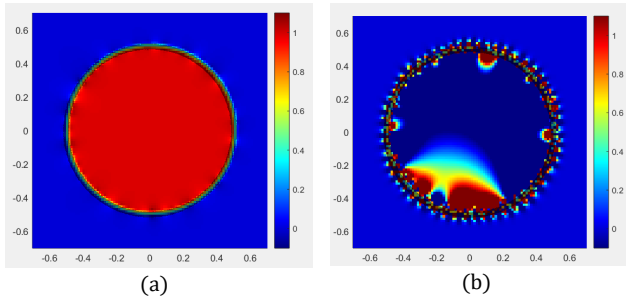

Fig. 1. Winding number field formed by a 2D circle of  $\sigma = 0.001$  with (a) and without (b) the regularization term  $R(P)$ .

Author's address:

© 2024

## B COMPARISONS WITH THE POINT PROJECTION METHOD

Our method aims to optimize the point positions for improving the winding clearness of the input point set. Both the input and output of our method are point clouds. In the original manuscript, the reconstruction method utilized in Section 6.2 serve as a way to showcase the quality of the denoised point clouds. However, an alternative approach for generating denoised point clouds involves applying an unoriented surface reconstruction method with a noise-adaptive parameter, followed by sampling or projecting the noisy point clouds onto the generated surface. We will illustrate the distinctions between our method and the projection-based method from three perspectives:

Firstly, surface reconstruction involves extracting the iso-surface from the implicit field. In cases where the computation fails to achieve consistent normal orientation or encounters difficulties with thin or complex features, the resulting surface may have missing structures compared to the original point cloud. When the noisy point cloud is projected onto the reconstructed surface, it also lead to missing regions in the results. In contrast, our method directly optimizes the point positions, effectively addressing this issue. Figure 2 provides a visual comparison between our method and the projection method. The surface is reconstructed using PGR [Lin et al. 2022] with a noise-adaptive parameter setting. The projected points are marked as “PGR Proj.” in this figure. From the first example, it can be observed that the projected point cloud loses details in thin structures due to incomplete reconstruction of the surface. Our method efficiently handles this situation. In the second example, the reconstructed surface not only exhibits missing features but also undergoes overall shrinkage comparing to the original point cloud. Therefore, the projected point cloud cannot accurately express the shape of the input.

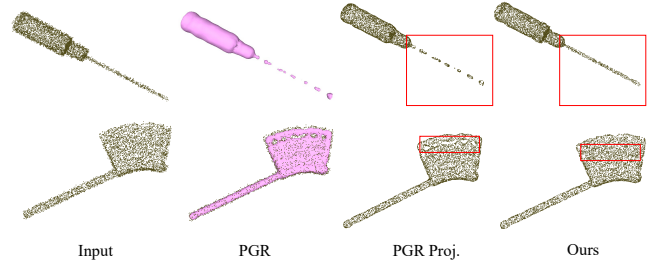

Fig. 2. Qualitative comparisons of our method with the point projection method. The surface is reconstructed by PGR with a noise-adaptive parameter setting.

Secondly, the denoised point clouds of our method lead to more complete surface reconstruction results compared with the original point clouds in many cases. This advantage has been demonstrated in Fig. 6 of the original manuscript, where iPSR [Hou et al. 2022] is utilized for surface reconstruction. We also provide results on PGR in Fig. 3 below to further illustrate this advantage.

Lastly, our approach introduces a differentiable point cloud optimization scheme that can be extended to the learning-based point processing, such as the diffusion-based generative model outlined in Section 5.2. Taking an alternative perspective, we extend PGR to a fully differentiable point-based form. The results presented in Section 6.3 also showcase the enhancements achieved by our method in both the point clouds and the reconstructed surfaces.

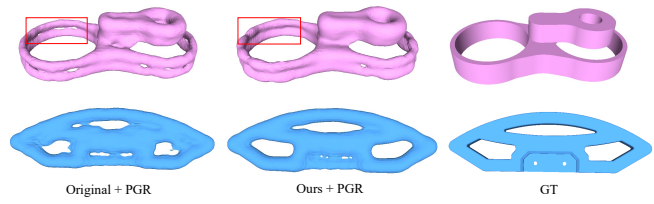

Fig. 3. Reconstruction of PGR (with a noise adaptive parameter setting) using the original input and the optimized point clouds from our method.

## REFERENCES

- Fei Hou, Chiyu Wang, Wencheng Wang, Hong Qin, Chen Qian, and Ying He. 2022. Iterative poisson surface reconstruction (iPSR) for unoriented points. *ACM Trans. Graph.* 41, 4 (2022), 128:1–128:13. <https://doi.org/10.1145/3528223.3530096>
- Siyu Lin, Dong Xiao, Zuoqiang Shi, and Bin Wang. 2022. Surface Reconstruction from Point Clouds without Normals by Parametrizing the Gauss Formula. *ACM Transactions on Graphics* 42, 2 (2022), 14:1–14:19.
